# Supplementary material for: Structural Pathways Supporting Swift Acquisition of New Visuo-Motor Skills
Source: arXiv:1605.04033 ancillary file (2016-10-24)
Supplement: Supplementary file 1 [file supplement.pdf]

## Supplementary Information

### Parietal and Occipital Regions Mediate Indirect Connectivity

In the main manuscript, we report an assessment of indirect connections between visual and motor systems. This analysis provides information about the strength of connectivity of distant regions through walks of length greater than one. However, it is also important to note that this analysis does not provide information about the exact paths that these walks take, or the influence that any particular intermediate region may hold on the structure or strength of the walk. To determine which intermediate nodes might influence these walks, we extend the notion of betweenness centrality to clusters of nodes. More specifically, we recall that the weighted betweenness centrality $g$ for a node $v$ is given by $g(v) = \frac{1}{(N-1)(N-2)} \sum_{a \neq v \neq b} \sigma_{ab}(v)$ where $\sigma_{ab}(v) := 1$ if $v$ lies along the shortest path from node $a$ to node $b$, and otherwise $\sigma_{ab}(v) := 0$ (Brandes, 2010). Then for clusters $A$ and $B$, $g_{AB}(v) = \frac{1}{|A||B|} \sum_{a \in A} \sum_{b \in B} \sigma_{ab}(v)$. We define the shortest paths using the inverse of connection strength $1/A$ as an estimate of distance (Goñi et al., 2014). With these definitions, we can compute $g_{AB}$ where $A$ and $B$ are respectively the sets of motor and visual regions, and $v$ is any node outside of these two clusters. Next, we studied the anatomical distribution of $g_{AB}$ by averaging values of $g_{AB}$ within each lobe while making sure to neglect the motor or visual areas in $A$ and $B$.

We find that parietal and occipital areas both have the largest mean average betweeness centrality. See Table 1. To test for the statistical significance of these effects, we performed a non-parametric permutation test in which betweenness centrality values were assigned to nodes uniformly at random without replacement. After 1000 such re-assignments, we computed the distributions of mean betweenness in each lobe, and compared the true values of betweenness centrality in each lobe to these permutation-based distributions. We observed that the mean betweenness centrality in the parietal and occipital lobes was significantly higher than expected under the null hypothesis: $p < 0.001$ for both lobes.

| Betweenness centrality, $g$ | Frontal | Limbic | Occipital | Parietal | Subcortical | Temporal |
|---|---|---|---|---|---|---|
| Mean | 0.0016 | 0.0164 | 0.0820 | 0.0607 | 0.0379 | 0.0152 |
| Standard deviation | 0.0030 | 0.0230 | 0.0677 | 0.0461 | 0.0588 | 0.0206 |

**Table 1. Betweenness centrality per lobe in shortest paths between motor and visual cortices.** Here we show the betweenness centrality averaged over all nodes within a lobe of the brain, for the shortest paths linking motor and visual cortices. Separate lines are given for mean and standard deviation.

## Temporal Stability of Structural Network Architecture Across Scans

In the main manuscript, we show that connection strength within a visual module of interest is strongly correlated with learning rate across 4 scanning sessions. Here, we consider the possibility that this correlation might change in a statistically meaningful way over the course of training. To test for this possibility, we performed an ANCOVA in which we modeled the scanning session as a covariate in the relationship between visual connection strength and learning rate. We found no significant effect of scanning session (see Fig. 1 and Table 2), suggesting that the relationship between connection strength and learning rate is stable over the course of our experiment.

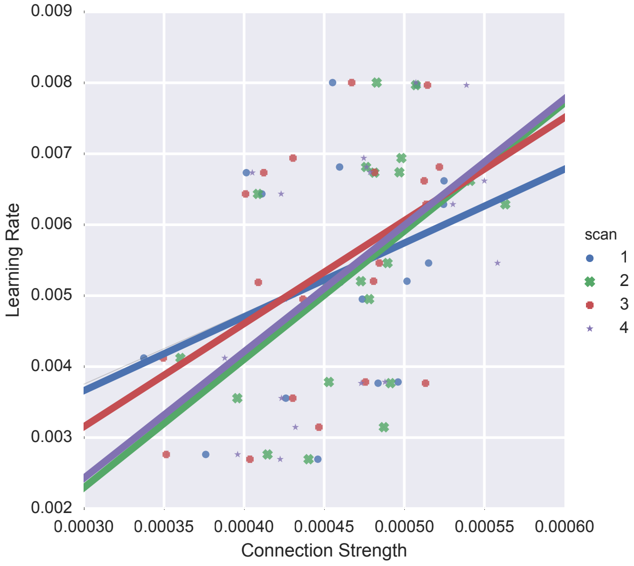


**Figure 1. Temporal Stability of Structural Network Architecture Across Scans.** Here we plot the relationship between visual connectivity and learning rate as a function of scanning session: scan 1 (blue circle), scan 2 (green cross), scan 3 (red square), and scan 4 (purple star). Lines show best fit for each scanning session separately.

## Learning Rate Predicted By Local and not Global Connectivity

In the main manuscript, we demonstrated that the strength of indirect walks between motor and visual areas was correlated with individual differences in learning. However, it is interesting to ask whether this finding is specifically driven by the local connectivity between motor and visual cortices, or whether it is driven by a global property of the entire graph (that is, connectivity patterns across the whole brain). To address this question, we examined the characteristic path length, which is calculated as the mean of all shortest paths: $l_G = \frac{1}{n(n-1)} \sum_{i \neq j} d(v_i, v_j)$ where $n$ is the number of nodes and $d(v_i, v_j)$ is the

| Source | d.f. | Sum Sq | Mean Sq | F | Prob>F |
|---|---|---|---|---|---|
| scan | 3 | 0 | 2.51803e-07 | 0.11 | 0.9556 |
| streamlines | 1 | 0.00005 | 4.52298e-05 | 19.27 | 0 |
| scan*streamlines | 3 | 0 | 6.04736e-07 | 0.26 | 0.8556 |
| Error | 69 | 0.00016 | 2.34703e-06 | | |

**Table 2. Results from an Analysis of Covariance.** We model the effect of scanning session as a covariate in the relationship between learning rate and visual connection strength. Importantly, we see no significant effect from the scanning session.

distance between nodes $i$ and $j$. We used $1/A$ as a distance metric between nodes (Goñi et al., 2014). We find no significant correlation between characteristic path length and learning rate ($r = -0.076$, $p = 0.75$), supporting the idea that our effect is localized to connectivity between motor and visual regions.

## Motor-to-Motor Connections Are Not Correlated with Learning Rate

While the analysis presented in the main manuscript demonstrated that average motor-to-motor connectivity strength was correlated with individual differences in learning rate, we nonetheless examined whether aggregating across all motor regions might be masking individual region pair effects. We repeated the same analysis as within visual cortex to examine individual edges and their relationship with learning rate. We found no significant edges after applying a false discovery rate correction for multiple comparisons. These results demonstrate that our findings are specific to direct visual connections, and to indirect connections between visual and motor areas.

## Low Structural Variability Within Subject

To further quantify the reproducibility of the structural connections that we study in the main manuscript, here perform an assessment of test-retest reliability. Specifically, we verify that connection strengths estimated from repeated scans of an individual subject showed significantly lower variance than scans of different subjects. To implement this analysis, we computed the mean of the per-edge variance in strength, both for each scan and for each subject. Next, we performed a $t$-test on the two groups (mean within-subject variance $= 4.63 \times 10^{-9}$, mean within-scan variance $= 1.18 \times 10^{08}$, $t = -24.13$, $p = 2.56 \times 10^{-17}$). These results confirm that between-scan variability is significantly lower than between-subject variability, indicating that we are well-powered to observe the structural differences between subjects.

### Data for a Single Week is Insufficient to Fit Model of Learning Rate

We were interested to determine whether we could fit learning rates to shorter periods, and thereby study individual differences in learning as they evolve at finer time scales. To address this question, we examined the periods between pairs of scans, and estimated the changes in learning rates over time. However, we found that stable estimates of learning rate were impossible to obtain without using the majority of the data for a given subject. We plot the size of the 95% confidence interval for the learning rate $\kappa$ and show that the estimate only stabilizes (i.e., displays narrow confidence intervals) after using half of the data (see Fig. 2). As our estimates of the learning rate parameter are on the order of $10^{-2}$, this is not an insignificant range. This fact precludes the possibility of fitting the learning rate in the periods between scans, which would at most contain a third of the available data. While individual subject estimates are not included, we mention that learning rate estimates show very erratic behavior when using less than half the data for many of the subjects.

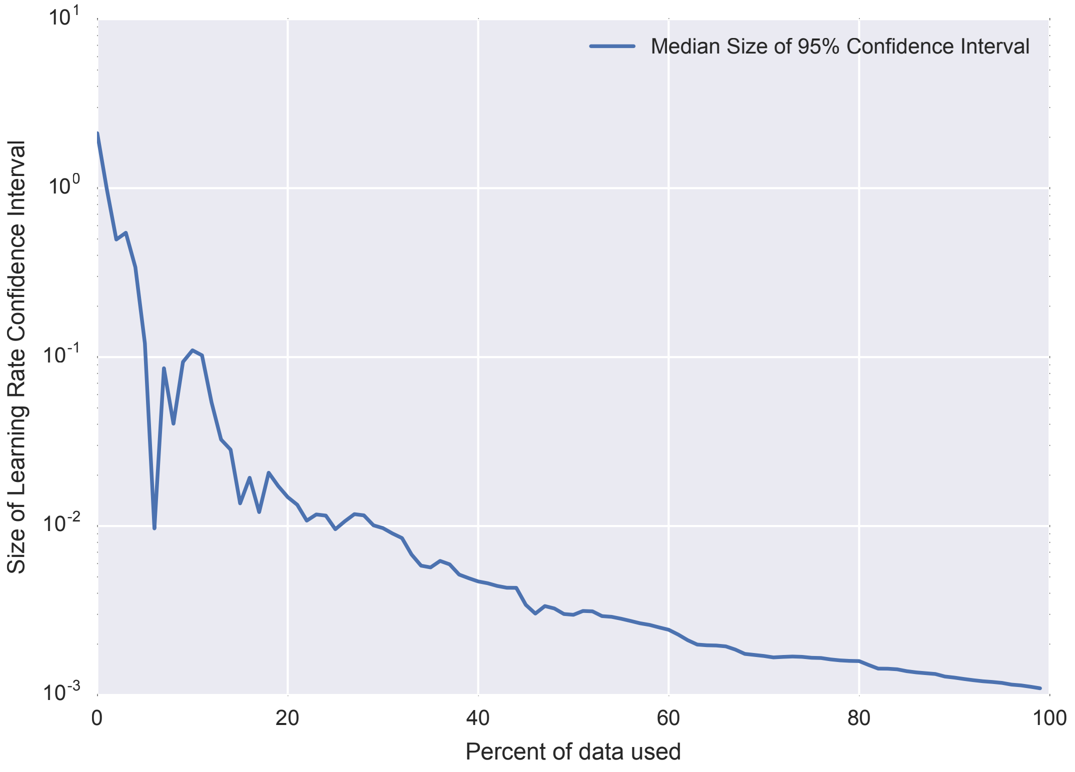


**Figure 2. Confidence Interval Size:** We plot the median size of the confidence interval across subjects for our learning rate parameter $\kappa$ as a function of the percent of the movement time data used. Use of small portions of the data lead to wide confidence intervals.

### Asymptotic Behavior of Walk Length Reveals Large-Scale Structure of Network

In the main manuscript, we demonstrate that individual differences in the strengths of walks of length greater than 1 between motor and visual cortices provide information about individual differences in learning rate. It is interesting to consider the structure of the matrix representing these longer walk lengths. Therefore, we provide a brief analysis of the asymptotic behavior of walks of increasingly high length on the structural adjacency matrix. Note that we compute walks using the matrix $S = D^{-\frac{1}{2}} A D^{-\frac{1}{2}}$ and $D = diag(d_i)$. Since $S$ is a symmetric matrix, we can write $S^n = U^T D^n U$ where $U$ is a matrix of eigenvectors of $S$. As $n$ approaches infinity, this becomes $u^T u$ where $u$ is the eigenvector of $S$ associated with the largest eigenvalue, and therefore representative of large-scale structure in the matrix. These observations support the notion that by studying longer walk lengths, we are studying the dynamics of large-scale structures in the human connectome, and moreover this large-scale structure is important for human learning.

### Alternative Indirect Connectivity Measures Show Similar Relationship to Learning Rate

Finally, we asked whether we could support our finding of the role of indirect connectivity in learning by demonstrating that related measures of indirect connectivity provided similar results. To address this question, we computed the indirect connectivity between motor and visual regions by means of the random walk measure used in the method called *Walktrap* (Pons and Latapy, 2006). For Walktrap, the distance between nodes $i$ and $j$ is given as $d(i,j) = \sqrt{\sum_k P^t_{i*} - P^t_{j*}{}^2 / d_k}$. We find that the random walk-based motor-visual connectivity correlates very strongly with learning, supporting our initial analysis ($r = 0.64$, $p = 0.002$). These results suggest that the observed effect is not unique to walk strength, but is more generally an effect of indirect connectivity.

## References


Brandes, U. (2010). A faster algorithm for betweenness centrality*. *Journal of Mathematical Sociology*.

Goñi, J., van den Heuvel, M. P., Avena-Koenigsberger, A., Velez de Mendizabal, N., Betzel, R. F., Griffa, A., Hagmann, P., Corominas-Murtra, B., Thiran, J.-P., and Sporns, O. (2014). Resting-brain functional connectivity predicted by analytic measures of network communication. *Proceedings of the National Academy of Sciences of the United States of America*, 111(2):833–838.

Pons, P. and Latapy, M. (2006). Computing Communities in Large Networks Using Random Walks. *Journal of Graph Algorithms and Applications*.
